# Supplementary material for: PAIR: Depiction-Invariant Representation Learning for Optical Chemical Structure Recognition
Source: arXiv:2611.40395 source file (2026-11-30)
Supplement: Supplementary file 1 [file X_suppl.tex]

\clearpage
\setcounter{page}{1}
\maketitlesupplementary

\section*{Structure-Aware Similarity Refinement}

Cross-view contrastive learning encourages depiction consistency
and discrimination between molecular identities. However, it
treats different molecules as negatives without explicitly
accounting for their structural relationships. We therefore
introduce a subsequent similarity refinement stage, initialized
from the contrastively trained PAIR checkpoint, to encourage
embedding similarities to reflect molecular structural similarity.

For each view $v \in \{r,s\}$, we compute the normalized
global representation as
\begin{equation}
g_{v,i}
=
\operatorname{normalize}
\left(
P_\omega\left(\operatorname{Pool}(Z_{v,i})\right)
\right).
\end{equation}
Given a mini-batch containing $B$ paired samples, the cross-view
embedding similarity is
\begin{equation}
S_{ij}=g_{r,i}^{\top}g_{s,j}.
\end{equation}
Let $f_i$ denote the binary molecular fingerprint of the
ground-truth structure $G_i$. We define the target structural
similarity using the Tanimoto coefficient:
\begin{equation}
T_{ij}
=
\frac{f_i^\top f_j}
{\|f_i\|_1+\|f_j\|_1-f_i^\top f_j}.
\end{equation}

We refine the embedding geometry by matching similarities
between different samples to their structural targets:
\begin{equation}
\mathcal{L}_{\mathrm{Tanimoto}}
=
\frac{1}{B(B-1)}
\sum_{i=1}^{B}
\sum_{\substack{j=1\\j\neq i}}^{B}
\left(S_{ij}-T_{ij}\right)^2.
\end{equation}
The diagonal terms are excluded because consistency between
paired depictions is already encouraged by the retained
cross-view contrastive objective. Since all ordered
off-diagonal pairs are included, the loss supervises both
real-to-rendered and rendered-to-real relationships.

During refinement, we jointly optimize
\begin{equation}
\mathcal{L}_{\mathrm{refine}}
=
\mathcal{L}_{\mathrm{recognition}}^{r}
+
\mathcal{L}_{\mathrm{recognition}}^{s}
+
\beta\mathcal{L}_{\mathrm{Tanimoto}}
+
\gamma\mathcal{L}_{\mathrm{contrast}},
\end{equation}
where $\beta$ and $\gamma$ control structural similarity
matching and cross-view contrastive supervision, respectively.
We freeze the image encoder and update the Q-Former,
projection head, residual fusion module, and SMILES decoder.
Hyperparameters and checkpoints are selected using
validation recognition performance.

This sequential design first establishes cross-depiction
correspondence and then refines the structural organization
of the learned representations. Tanimoto supervision provides
graded relationships between molecules, allowing structurally
related molecules to have similar representations without
requiring identical embeddings. The retained contrastive
objective encourages molecular identity discrimination,
while recognition supervision constrains the representation
to preserve distinctions needed for exact SMILES decoding.
Together, these objectives aim to balance depiction consistency,
structural similarity, and chemical fidelity.
